# Supplementary material for: WorldBridge: Bridging Video and Action for Task Generalization in World Action Models
Source: arXiv:2610.40748 source file (2026-11-06)
Supplement: Supplementary file 1 [file 99_appendix.tex]

\section{Appendix}
